# Supplementary material for: A Learned Cache Eviction Framework with Minimal Overhead
Source: arXiv:2301.11886 source file (2023-01-27)
Supplement: Supplementary file 1 [file appendix.tex]

\section{Full Structured Proof}

Something

\section{Additional Details Cut for Space}

\section{Full Experimental Details}

\section{Full Related Work Discussion}

An ideal, full related work discussion has a dedicated paragraph per
related paper.  It might have more than one paragraph for the most
closely related work.  A great way to organize your thoughts on
related work (or at least the competing work subset of related work)
is with a comparison table, e.g.,
Table~\ref{tbl:rcc_related}.\footnote{\url{http://www.tablesgenerator.com/latex\_tables}
  takes a gdoc or excel spreadsheet and makes it a latex table.}

\onecolumn
\begin{sidewaystable}
%\begin{table*}[]
\centering
\caption{Rococo related work comparison table}
\label{tbl:rcc_related}
\begin{tabular}{llllllllll}
                             & \textbf{Isolation level}& \textbf{Concurrency Control} & \textbf{Pre} & \textbf{Txn type}                                                                            & \textbf{Extra Txn} & \textbf{Extra Mech}  & \textbf{P/C}      & \textbf{contended abort} & \textbf{user-initiated abort} \\
MegaStore/Spanner            & strict-serializability  & 2PL + 2PC                                         & no  & x-shot                                                                              & read-only &                        & parallel & yes             & yes                  \\
H-Store/VoltDB               & strict-serializability  & none                                              & yes & single-site                                                                         & general   & OCC + 2PC (lock all)   & parallel & yes             & yes                  \\
H-Store + OCC                & strict-serializability  & OCC+2PC                                           & yes & X-shot                                                                              &           &                        & parallel & yes             & yes                  \\
Sinfornia                    & strict-serializability  & 2PC                                               & no  & value-two-shot                                                                      &           &                        & parallel & yes             & first shot           \\
Sinfornia + OCC              & strict-serializability  & 2PC+OCC                                           & no  & X-shot                                                                              &           &                        & parallel & yes             & yes                  \\
COPS                         & causal                  & dependency tracking                               & no  & read-only one-shot                                                                  &           &                        & parallel & yes             & no                   \\
Eiger                        & causal                  & lamport timestamp                                 & no  & read-only one-shotwrite-only one-shot                                               &           &                        & parallel & yes             & no                   \\
Lynx                         & serializability         & serializability                                   & yes & SC-acyclic                                                                          & All       & origin orderingocc/2pl & chain    & no              & first site           \\
Lynx+Origin Ordering         & serializability         & serializability                                   & yes & SC-acyclic orcycle starts from the same server                                      &           &                        & chain    & no              & first site           \\
Lynx+Origin Ordering+2PL/OCC & serializability         & serializability                                   & yes & SC-acyclic, orcycle starts from the same server, all other cycles solved by 2PL/OCC &           &                        & chain    & yes             & first site           \\
Calvin                       & strict-serializability  & pre-ordering locking                              & no  & value-two-shot                                                                      & X phase   & occ                    & parallel & no              & first shot           \\
Calvin + OCC                 & strict-serializability  & pre-ordering locking                              & no  & X-shot                                                                              &           &                        & parallel & yes             & yes                  \\
Granola                      & serializability         & timestamp ordering                                & no  & value-two-shot                                                                      & two-phase & 2pl                    & parallel & no              & no                   \\
Granola + 2PL                & serializability         & timestamp+2PL+2PC                                 & no  & X-shot                                                                              &           &                        & parallel & yes             & yes                  \\
Percolator                   & snapshot isolation      & occ + 2pc                                         & no  & general                                                                             &           &                        & parallel & yes             & yes                  \\
Warp                         & strict-serializability? & occ +dependency tracking                          & no  & value-two-shot                                                                      &           &                        & chain    & yes             & yes                  \\
Walt                         & psi                     & occ + 2pc                                         & no  & X-shot                                                                              & ?         & ?                      & parallel & yes             & yes                  \\
epaxos-strict                & strict-serializability  & dependency tracking + reordering                  & no  & replicated single-site                                                              &           &                        & parallel & no              & yes                  \\
Rococo                       & strict-serializability  & dependency tracking + reordering                  & yes & I-I SC-acyclic                                                                      &           &                        & parallel & no              & no                   \\
Rococo+                      & strict-serializability  & dependency tracking + reordering + 2PL            & yes & all I-I SC-cycles are solved by OCC/2PL                                             &           &                        & parallel & yes             & no                   \\
Rococo*                      & strict-serializability  & dependency tracking + reordering + cascade aborts & yes & X-shot                                                                              &           &                        & parallel & yes             & yes                  \\
OCC in Rococo(+,*)           & strict-serializability  & OCC                                               & yes & read-only X-shot                                                                    &           &                        & parallel & yes             & yes                 
\end{tabular}
%\end{table*}
\end{sidewaystable}
\twocolumn
